# Supplementary material for: Dynamic Domain Adaptation for Efficient Inference
Source: arXiv:2103.16403 source file (2021-03-26)
Supplement: Supplementary file 1 [file appendix.tex]

\section*{Supplementary Material for Paper ID 1284}

\subsection{Algorithm of DDA}
Details of the overall training procedure of the proposed DDA is shown in Algorithm \ref{alg:Framwork}. In step 1, we deploy cross-entropy and domain confusion loss on each exit. In step 2, we firstly assign the confidence score $v_j$ for each target sample $\x_t^j$ to build a score set. Then we sort the score set by values and select highly confident target samples with pseudo labels, during which we adopt the novel class-balance strategy. Finally those selected samples are randomly assigned to different classifiers to provide additional cross-entropy loss.

\begin{algorithm}[!htbp]
  \small
  \caption{\small Dynamic Domain Adaptation.}
  \label{alg:Framwork}
  \begin{algorithmic} [1]
    \REQUIRE
      Source domain $\{\left(\x_s^i,y_s^i\right)\}_{i=1}^{N_s}$; Target domain $\{\x_t^j\}_{j=1}^{N_t}$; Parameters $\mu$, $\alpha$ and $\beta$; Max iteration: $I$
    \ENSURE
      trained model $G=\{f_k(\cdot; \theta_k)|_{k=1}^{K}\}$
    \begin{enumerate}
        \item[\textbf{Step 1}] Adaptive Network with Domain Confusion Learning:
    \end{enumerate}
        \STATE Compute $\Lm_s$ and $\Lm_d$ with SGD optimization;
    \begin{enumerate}
        \item[\textbf{Step 2}] Target Class-balanced Self-training:
    \end{enumerate}
        \FOR{$i=1,2,\cdots,I$}
            \STATE For each $\x_t^j$, calculate $\bar{\p}_t^j$ and confidence score $v_j$;
            \STATE Sort confidence score set $V$;
            \STATE For each class $c$, calculate threshold $\lambda_c$;
            \STATE Construct target self-training set $U$;
            \STATE Randomly assign samples in $U$ to different classifiers;
            \STATE Proceed target class-balanced self-training, compute $\mathcal{L}_{s}$, $\mathcal{L}_{t}$ and $\Lm_d$ with SGD optimization;
        \ENDFOR
  \end{algorithmic}
\end{algorithm}

\subsection{Experimental details}

\textbf{Inductive learning on DomainNet.} Different from Office31 and VisDA-2017, we utilize training set, validation set, and in addition the test set on DomainNet.
Thus, we implement inductive learning where the test set would not be used in the network training.

\textbf{Training details.}
We adopt mini-batch stochastic gradient descent (SGD) optimization with a momentum of 0.9 and the same learning rate annealing strategy as in~\cite{DA_bp}.
All samples are cropped into 224$\times$224 and the batch size for each domain is 36.
In class-balanced self-training phase, we use the batch formulation method described in~\cite{iCAN}, which specifies the proportion of target pseudo labels within a training batch. 

\subsection{Additional Experimental Results}
\begin{figure*}[htbp]
    \centering
    \includegraphics[width=0.98\textwidth]{figures/fig_addtion_anytime.pdf}
    \caption{Anytime classification results on DomainNet (\textbf{pnt}$\rightarrow$\textbf{rel}, \textbf{inf}$\rightarrow$\textbf{rel}, \textbf{qdr}$\rightarrow$\textbf{rel}, \textbf{skt}$\rightarrow$\textbf{rel}).}
    \label{anytime_classification}%\vspace{-5mm}
\end{figure*}
\begin{figure*}[htbp]
    \centering
    \includegraphics[width=0.98\textwidth]{figures/fig_addtion_budget.pdf}
    \caption{Budgeted classification results on DomainNet (\textbf{pnt}$\rightarrow$\textbf{rel}, \textbf{inf}$\rightarrow$\textbf{rel}, \textbf{qdr}$\rightarrow$\textbf{rel}, \textbf{skt}$\rightarrow$\textbf{rel}).}
    \label{budgeted_classification}%\vspace{-5mm}
\end{figure*}

\subsection{Anytime and Budgeted prediction results on DomainNet}
We provide more results on DomainNet under anytime prediction and budgeted classification scenarios, respectively.
We evaluate them on four tasks that are from different source domain to the ``real'' domain.
Here we use DANN~\cite{DANN} as the adversarial objective and adopt the experimental settings identical to the former experiment.
As shown in Fig. \ref{anytime_classification}, DDA consistently outperforms other baseline methods by a large margin and meanwhile saves computational resources.
